# Supplementary material for: High Order Residual Distribution Conservative Finite Difference HWENO Scheme for Steady State Problems
Source: arXiv:2104.06731 source file (2021-11-04)
Supplement: Supplementary file 2 [file acknowledgement.tex]

\section*{Acknowledgments}
